# Supplementary material for: Contextual Bandits with Online Neural Regression
Source: arXiv:2312.07145 source file (2023-12-12)
Supplement: Supplementary file 2 [file Appendix.tex]

% \section{Neural Online Regression with ReLu activation}
\label{sec:Appendix_reg_relu}

% \section{Neural Contextual Bandits with ReLu activation (Section)}
% \label{sec:Appendix_C}

% \subsection{Regret for Squared Loss}
% \label{sec:Appendix_C1}

% \subsection{Regret for KL loss}
% \label{sec:Appendix_C2}
